# Supplementary material for: Efficient Mutation Testing via Pre-Trained Language Models
Source: arXiv:2301.03543 source file (2023-01-09)
Supplement: Supplementary file 1 [file appendix.tex]

\onecolumn
\appendix[Extra examples]

\begin{table*}[!htp]
\centering
\caption{This table presents more mutants generated by {\OurTool} for the faults Cli\_10, Csv\_15 and Csv\_16.}
% \resizebox{\textwidth}{!}{
\begin{tabular}{l}
\toprule
{\textbf{BugID:} Cli\_10. \hspace*{1cm} \textbf{Class:} Parser.java} \\
\midrule
\begin{lstlisting}[language=diff]
@@ MUTANT: -306,7 +306,7 @@ 
- if (getRequiredOptions().size() > 0)
+ if (getRequiredOptions().size() > 2)

@@ MUTANT: -321,7 +321,7 @@
- throw new MissingOptionException(buff.substring(0, buff.length() - 2));
+ throw new MissingOptionException(buff.substring(0, buff.length()+2));
\end{lstlisting}
\\
\midrule
{\textbf{BugID:} Csv\_15. \hspace*{1cm} \textbf{Class:} CSVFormat.java} \\
\midrule
\begin{lstlisting}[language=diff]
@@ MUTANT: -790,7 +790,7 @@ 
public String[] getHeaderComments() {
-        return headerComments != null ? headerComments.clone() : null;
+        return headerComments==null ? headerComments.clone() : null;
}

@@  MUTANT: -879,7 +879,7 @@ 
    public boolean getTrailingDelimiter() {
-       return trailingDelimiter;
+       return true;
  }

@@ MUTANT: -1081,7 +1081,7 @@ 
- charSequence = value instanceof CharSequence ? (CharSequence) value : value.toString();
+ charSequence = value instanceof Object ? (CharSequence) value : value.toString();

@@ MUTANT: -1726,7 +1726,7 @@ 
 return new CSVFormat(delimiter, quoteCharacter, quoteMode, commentMarker, escapeCharacter,
- ignoreSurroundingSpaces, ignoreEmptyLines, recordSeparator, nullString, headerComments, header,
+ ignoreSurroundingSpaces, ignoreEmptyLines, null, nullString, headerComments, header,
   skipHeaderRecord, allowMissingColumnNames, ignoreHeaderCase, trim, trailingDelimiter, autoFlush);
\end{lstlisting}
\\
\midrule
{\textbf{BugID:} Csv\_16. \hspace*{1cm} \textbf{Class:} CSVParser.java} \\
\midrule
\begin{lstlisting}[language=diff]
@@ MUTANT: -362,7 +362,7 @@ 
-        final String input = this.reusableToken.content.toString();
+        final String input = this.toString();

@@ MUTANT: -557,7 +557,7 @@ 
-            if (next == null) {
+            if (current == null) {

@@ MUTANT: -363,7 +363,7 @@ 
-        final String inputClean = this.format.getTrim() ? input.trim() : input;
+        final String inputClean = this.format.getTrim() ? input.trim() : "";

@@ MUTANT: -463,7 +463,7 @@ 
-        if (formatHeader != null) {
+        if (format != null) {

@@ MUTANT: -463,7 +463,7 @@ 
-        if (formatHeader != null) {
+        if (this != null) {

@@ MUTANT: -546,7 +546,7 @@ 
-            return this.current != null;
+            return this != null;
\end{lstlisting}
\\
\bottomrule
\end{tabular}
% }
\label{tab:extra-mutants}
\end{table*}
